# Supplementary material for: Micromagnetic simulations of magnetoelastic spin wave excitation in scaled magnetic waveguides
Source: arXiv:1708.06428 source file (2017-08-21)
Supplement: Supplementary file 1 [file Supplementary_Information.pdf]

**Supplementary Information for "Micromagnetic simulations of magnetoelastic spin wave excitation in scaled magnetic waveguides"**

Rutger Duflou,[1,2] Florin Ciubotaru,[1,a)] Adrien Vaysset,[1] Marc Heyns,[1,2] Bart Sorée,[1,2,3] Iuliana P. Radu,[1] and Christoph Adelmann[1,b)]

[1)] *Imec, B-3001 Leuven, Belgium*

[2)] *KU Leuven, Faculteit Ingenieurswetenschappen, B-3001 Leuven, Belgium*

[3)] *Universiteit Antwerpen, Departement Fysica, B-2000 Antwerpen, Belgium*

[a)] Electronic mail: Florin.Ciubotaru@imec.be

[b)] Electronic mail: Christoph.Adelmann@imec.be

# I. MAGNETOELASTIC TORQUE

The torque $\boldsymbol{\tau} = \mu_0 \boldsymbol{M} \times \boldsymbol{H}$ exerted on magnetization $\boldsymbol{M}$ by the effective magnetoelastic field, as given by Eq. (2) in the letter, can be expressed by

$$\begin{aligned}\boldsymbol{\tau} &= \mu_0 \boldsymbol{M} \times \boldsymbol{H} \\ &= \begin{pmatrix} 2B_1 m_y m_z(\varepsilon_{yy} - \varepsilon_{zz}) + B_2(m_z m_x \varepsilon_{xy} - m_x m_y \varepsilon_{zx} + (m_z^2 - m_y^2)\varepsilon_{yz}) \\ 2B_1 m_z m_x(\varepsilon_{zz} - \varepsilon_{xx}) + B_2(m_x m_y \varepsilon_{yz} - m_y m_z \varepsilon_{xy} + (m_x^2 - m_z^2)\varepsilon_{zx}) \\ 2B_1 m_x m_y(\varepsilon_{xx} - \varepsilon_{yy}) + B_2(m_y m_z \varepsilon_{zx} - m_z m_x \varepsilon_{yz} + (m_y^2 - m_x^2)\varepsilon_{xy}) \end{pmatrix}\end{aligned} \tag{S1}$$

# II. EXPLICIT FORMS OF THE STRAIN TENSORS

In all simulations, oscillation strain tensors with $\boldsymbol{\varepsilon}(t) = \boldsymbol{\varepsilon} \times \exp(2\pi i f t)$ were used. The magnetoelastic torque above is zero for hydrostatic strain $\boldsymbol{\varepsilon} = \varepsilon_0 \boldsymbol{I}$, which can be used to simplify the tensors. Below, we give explicit expressions of the amplitude tensors $\boldsymbol{\varepsilon}$ for the different geometries. Strain tensors were calculated for piezoelectric elements with top contacts as well as side contacts using the assumption that no shear strain components are present. The strain tensors are therefore of the form

$$\varepsilon = \begin{pmatrix} \varepsilon_{xx} & 0 & 0 \\ 0 & \varepsilon_{yy} & 0 \\ 0 & 0 & \varepsilon_{zz} \end{pmatrix} \tag{S2}$$

The strain components are calculated from the equations describing the force equilibrium between the piezoelectric layer and the magnetostrictive layer and the relation between the strain components in both layers. To solve these equations the following dimensions were used: width of the piezoelectric pillar $w = 200\,\mathrm{nm}$, length of the pillar $l = 200\,\mathrm{nm}$, height of the pillar $h_{\mathrm{PZT}} = 80\,\mathrm{nm}$, thickness of the magnetostrictive layer underneath the pillar $h_{\mathrm{mag}} = 10\,\mathrm{nm}$. Furthermore the following material properties were used: piezoelectric constants $d_{31} = -1.71 \times 10^{-10}$ $\mathrm{C\,N^{-1}}$ and $d_{33} = 3.74 \times 10^{-10}$ $\mathrm{C\,N^{-1}}$ and stiffness tensors equal to the inverse of the compliance tensors

$$s_{\mathrm{PZT}} = \begin{bmatrix} 16.4 & -5.74 & -7.22 & 0 & 0 & 0 \\ -5.74 & 16.4 & -7.22 & 0 & 0 & 0 \\ -7.22 & -7.22 & 18.8 & 0 & 0 & 0 \\ 0 & 0 & 0 & 47.5 & 0 & 0 \\ 0 & 0 & 0 & 0 & 47.5 & 0 \\ 0 & 0 & 0 & 0 & 0 & 44.3 \end{bmatrix}$$

$$s_{\mathrm{mag}} = \begin{bmatrix} \frac{1}{E} & -\frac{\nu}{E} & -\frac{\nu}{E} & 0 & 0 & 0 \\ -\frac{\nu}{E} & \frac{1}{E} & -\frac{\nu}{E} & 0 & 0 & 0 \\ -\frac{\nu}{E} & -\frac{\nu}{E} & \frac{1}{E} & 0 & 0 & 0 \\ 0 & 0 & 0 & \frac{2(1+\nu)}{E} & 0 & 0 \\ 0 & 0 & 0 & 0 & \frac{2(1+\nu)}{E} & 0 \\ 0 & 0 & 0 & 0 & 0 & \frac{2(1+\nu)}{E} \end{bmatrix} \tag{S3}$$

The compliance tensor of the magnetostrictive material corresponds to that of an isotropic material. The Young's modulus is taken equal to 113 GPa, the same as for permalloy, and the Poisson ratio is taken to be 0.3. Finally, it is assumed a voltage of $V = 1\,\mathrm{V}$ is applied over the gold contacts.

## A. Top contact

For the inducer with a top contact, the strain components are the result of the following six equations

$$\varepsilon_{xx,\mathrm{PZT,stress}} + d_{31}V/h_{\mathrm{PZT}} = \varepsilon_{xx,\mathrm{mag}} \tag{S4}$$

$$\varepsilon_{yy,\mathrm{PZT,stress}} + d_{31}V/h_{\mathrm{PZT}} = \varepsilon_{yy,\mathrm{mag}} \tag{S5}$$

$$\sigma_{xx,\mathrm{PZT}}h_{\mathrm{PZT}}w + \sigma_{xx,\mathrm{mag}}h_{\mathrm{mag}}w = 0 \tag{S6}$$

$$\sigma_{yy,\mathrm{PZT}}h_{\mathrm{PZT}}l + \sigma_{yy,\mathrm{mag}}h_{\mathrm{mag}}l = 0 \tag{S7}$$

$$(c_{31,\mathrm{PZT}}\varepsilon_{xx,\mathrm{PZT,stress}} + c_{32,\mathrm{PZT}}\varepsilon_{yy,\mathrm{PZT,stress}} + c_{33,\mathrm{PZT}}\varepsilon_{zz,\mathrm{PZT,stress}}) = 0 \tag{S8}$$

$$(c_{31,\mathrm{mag}}\varepsilon_{xx,\mathrm{mag}} + c_{32,\mathrm{mag}}\varepsilon_{yy,\mathrm{mag}} + c_{33,\mathrm{mag}}\varepsilon_{zz,\mathrm{mag}}) = 0 \tag{S9}$$

The first two equations describe the fact that the normal strain components in the $x$- and $y$-direction are the same for the piezoelectric layer and the magnetostrictive layer. The former

has two contributions, one from stress and one from the piezoelectric properties, while the latter is only due to stress. The next two equations describe the force equilibrium between both layers. The last two equations describe the fact that the pillar and hence both layers are free to extend in z-direction and hence have a normal stress component equal to zero in this direction. Solving these six equations results in the following strain tensor for the magnetostrictive layer

$$\varepsilon = \begin{bmatrix} -0.001759 & 0 & 0 \\ 0 & -0.001759 & 0 \\ 0 & 0 & 0.001508 \end{bmatrix} \tag{S10}$$

It can be seen that $\varepsilon_{xx} = \varepsilon_{yy} \neq \varepsilon_{zz}$. Subtracting a hydrostatic strain, leads to a simplified effective strain tensor of the form

$$\varepsilon_{\text{eff}} = \begin{pmatrix} 0 & 0 & 0 \\ 0 & 0 & 0 \\ 0 & 0 & \varepsilon_{zz} \end{pmatrix} \tag{S11}$$

Therefore, this situation is is referred to as a uniaxial normal out-of-plane strain in the main paper.

## B. Side contacts

In the case of side contacts, the six equations are the same except for the fact that now the electric field and the polarization of the piezoelectric layer are in the y-direction. This causes Eq. (S4) and Eq. (S5) to become

$$\varepsilon_{xx,\text{PZT,stress}} + d_{31} V/w = \varepsilon_{xx,\text{mag}} \tag{S12}$$

$$\varepsilon_{yy,\text{PZT,stress}} + d_{33} V/w = \varepsilon_{yy,\text{mag}} \tag{S13}$$

Solving these equations results in the following strain tensor

$$\varepsilon = \begin{pmatrix} -0.000657 & 0 & 0 \\ 0 & 0.001473 & 0 \\ 0 & 0 & -0.000350 \end{pmatrix} \tag{S14}$$

It can be seen that $\varepsilon_{xx} \neq \varepsilon_{yy} \neq \varepsilon_{zz}$. Subtracting a hydrostatic strain, leads to a simplified effective strain tensor of the form

$$\varepsilon_{\text{eff}} = \begin{pmatrix} -\varepsilon_{xx} & 0 & 0 \\ 0 & \varepsilon_{yy} & 0 \\ 0 & 0 & 0 \end{pmatrix} \tag{S15}$$

Therefore, this is referred to as a biaxial normal in-plane strain in the main paper.

## C. Rotated pillar

The strain tensor of a rotated pillar with side contacts is assumed to be equal to the strain tensor in Eq. (S15) but rotated by 45°. Rotation of a vector by $\theta$ is achieved by the following transformation matrix

$$A = \begin{bmatrix} \cos\theta & -\sin\theta & 0 \\ \sin\theta & \cos\theta & 0 \\ 0 & 0 & 1 \end{bmatrix} \tag{S16}$$

Since the strain is represented by a tensor, rotation by $\theta$ is achieved by

$$\varepsilon = A\varepsilon' A^T \tag{S17}$$

Using the strain tensor in Eq. (S15) and setting $\theta$ to 45°, this results in

$$\varepsilon = \begin{pmatrix} 0.000408 & -0.001065 & 0 \\ -0.001065 & 0.000408 & 0 \\ 0 & 0 & -0.000350 \end{pmatrix} \tag{S18}$$

Subtracting again a hydrostatic strain then leads to the simplified effective strain tensor

$$\varepsilon_{\text{eff}} = \begin{pmatrix} 0 & \varepsilon_{xy} & 0 \\ \varepsilon_{xy} & 0 & 0 \\ 0 & 0 & \varepsilon_{zz} \end{pmatrix} \tag{S19}$$

Since the shear strain components are larger and have a much more significant influence than the normal out-of-plane strain component, this case is referred to as shear in-plane strain in the main paper.

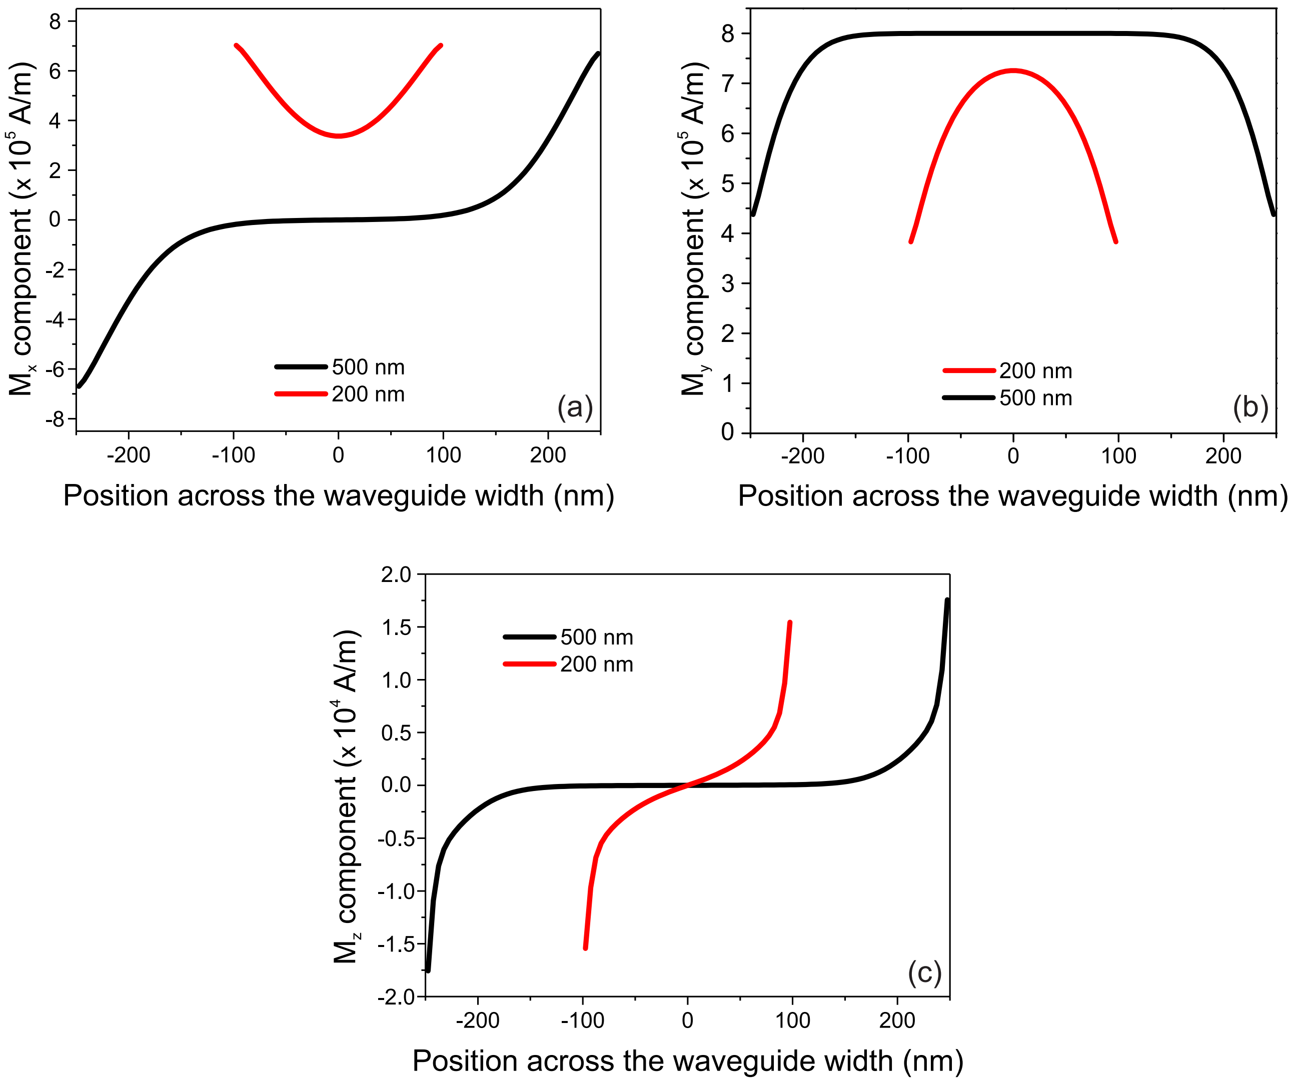


FIG. S1. Components of the equilibrium magnetization for both simulated structures of 200 nm and 500 nm width, respectively. An external transverse (along the $y$-direction) magnetic bias field of 50 mT was applied.
